# Supplementary material for: Ranking Policy Gradient
Source: arXiv:1906.09674 source file (2019-11-26)
Supplement: Supplementary file 1 [file sec_appendix_explore.tex]

% !TEX ROOT=./main.tex

\subsection{Exploration Efficiency}
\label{subsec:app:ee}

% \lkxcom{Goal: defense the attack from those aspects. }
% \begin{itemize}
% \item No theoretically analysis on sample complexity.
%     \item Talk about the sample-efficiency, but no exploration method specified. 
%     \item The sufficient number of different near-optimal trajectories collected is heuristic. 
% \end{itemize}

The proposed off-policy learning framework indicates the sample complexity is
related to exploration efficiency and supervised learning efficiency.  Given a
specific MDP, the exploration efficiency of an exploration strategy  can be
quantified by how frequently we can encounter different (near)-optimal
trajectories in the first $k$ episodes.  The supervised learning efficiency
under the probably approximately correct framework~\cite{valiant1984theory} is
how many samples we need to collect so that we can achieve good generalization
performance with high probability. Jointly consider the efficiency in two
stages, we can theoretically analyze the sample complexity of the proposed
off-policy learning framework, which will be provided in the long version of
this work. 

Improving exploration efficiency is not the focus of this work. In general,
exploration efficiency is highly related to the properties of MDP, such as
transition probabilities, horizon, action dimension, etc.  The exploration
strategy should be designed according to certain  domain knowledge of the MDP
to improve the efficiency. Therefore, we did not specify our exploration
strategy but adopt the state-of-the-art to conduct exploration.

% v1
% Indicated by the proposed off-policy learning framework, the exploration efficiency should be
% able to quantify how frequently we encounter the different (near)-optimal trajectories given
% a certain number of interactions with the environment. The more frequently we encounter
% different near-optimal trajectories, the higher the exploration efficiency. 
% Furthermore, the exploration efficiency is highly related to the dynamics of MDP. 
% Same exploration method will have very different exploration efficiency in different
% MDPs. In this work, we did not focus on how does a exploration method for certain MDP
% affects the sample efficiency. We empirically adopt the state-of-the-art as our exploration method.
% The theoretical analysis of sample complexity will be provided in the long version of this work.
% We briefly state here without providing further explanation, 
% the number of different near-optimal trajectories (sample size) needed is related to 
% our requirement on the final
% performance (determined by near-optimal trajectory reward threshold $c$), the dynamics
% of MDP, the sample complexity of supervised learning, and the exploration efficiency.
