# Supplementary material for: Ranking Policy Gradient
Source: arXiv:1906.09674 source file (2019-11-26)
Supplement: Supplementary file 2 [file sec_appendix_example.tex]

% !TEX ROOT=./main.tex

\section{A Running Example}
\label{sec:rpg:example}

\begin{figure}
\centering
	\includegraphics[width=0.5\textwidth]{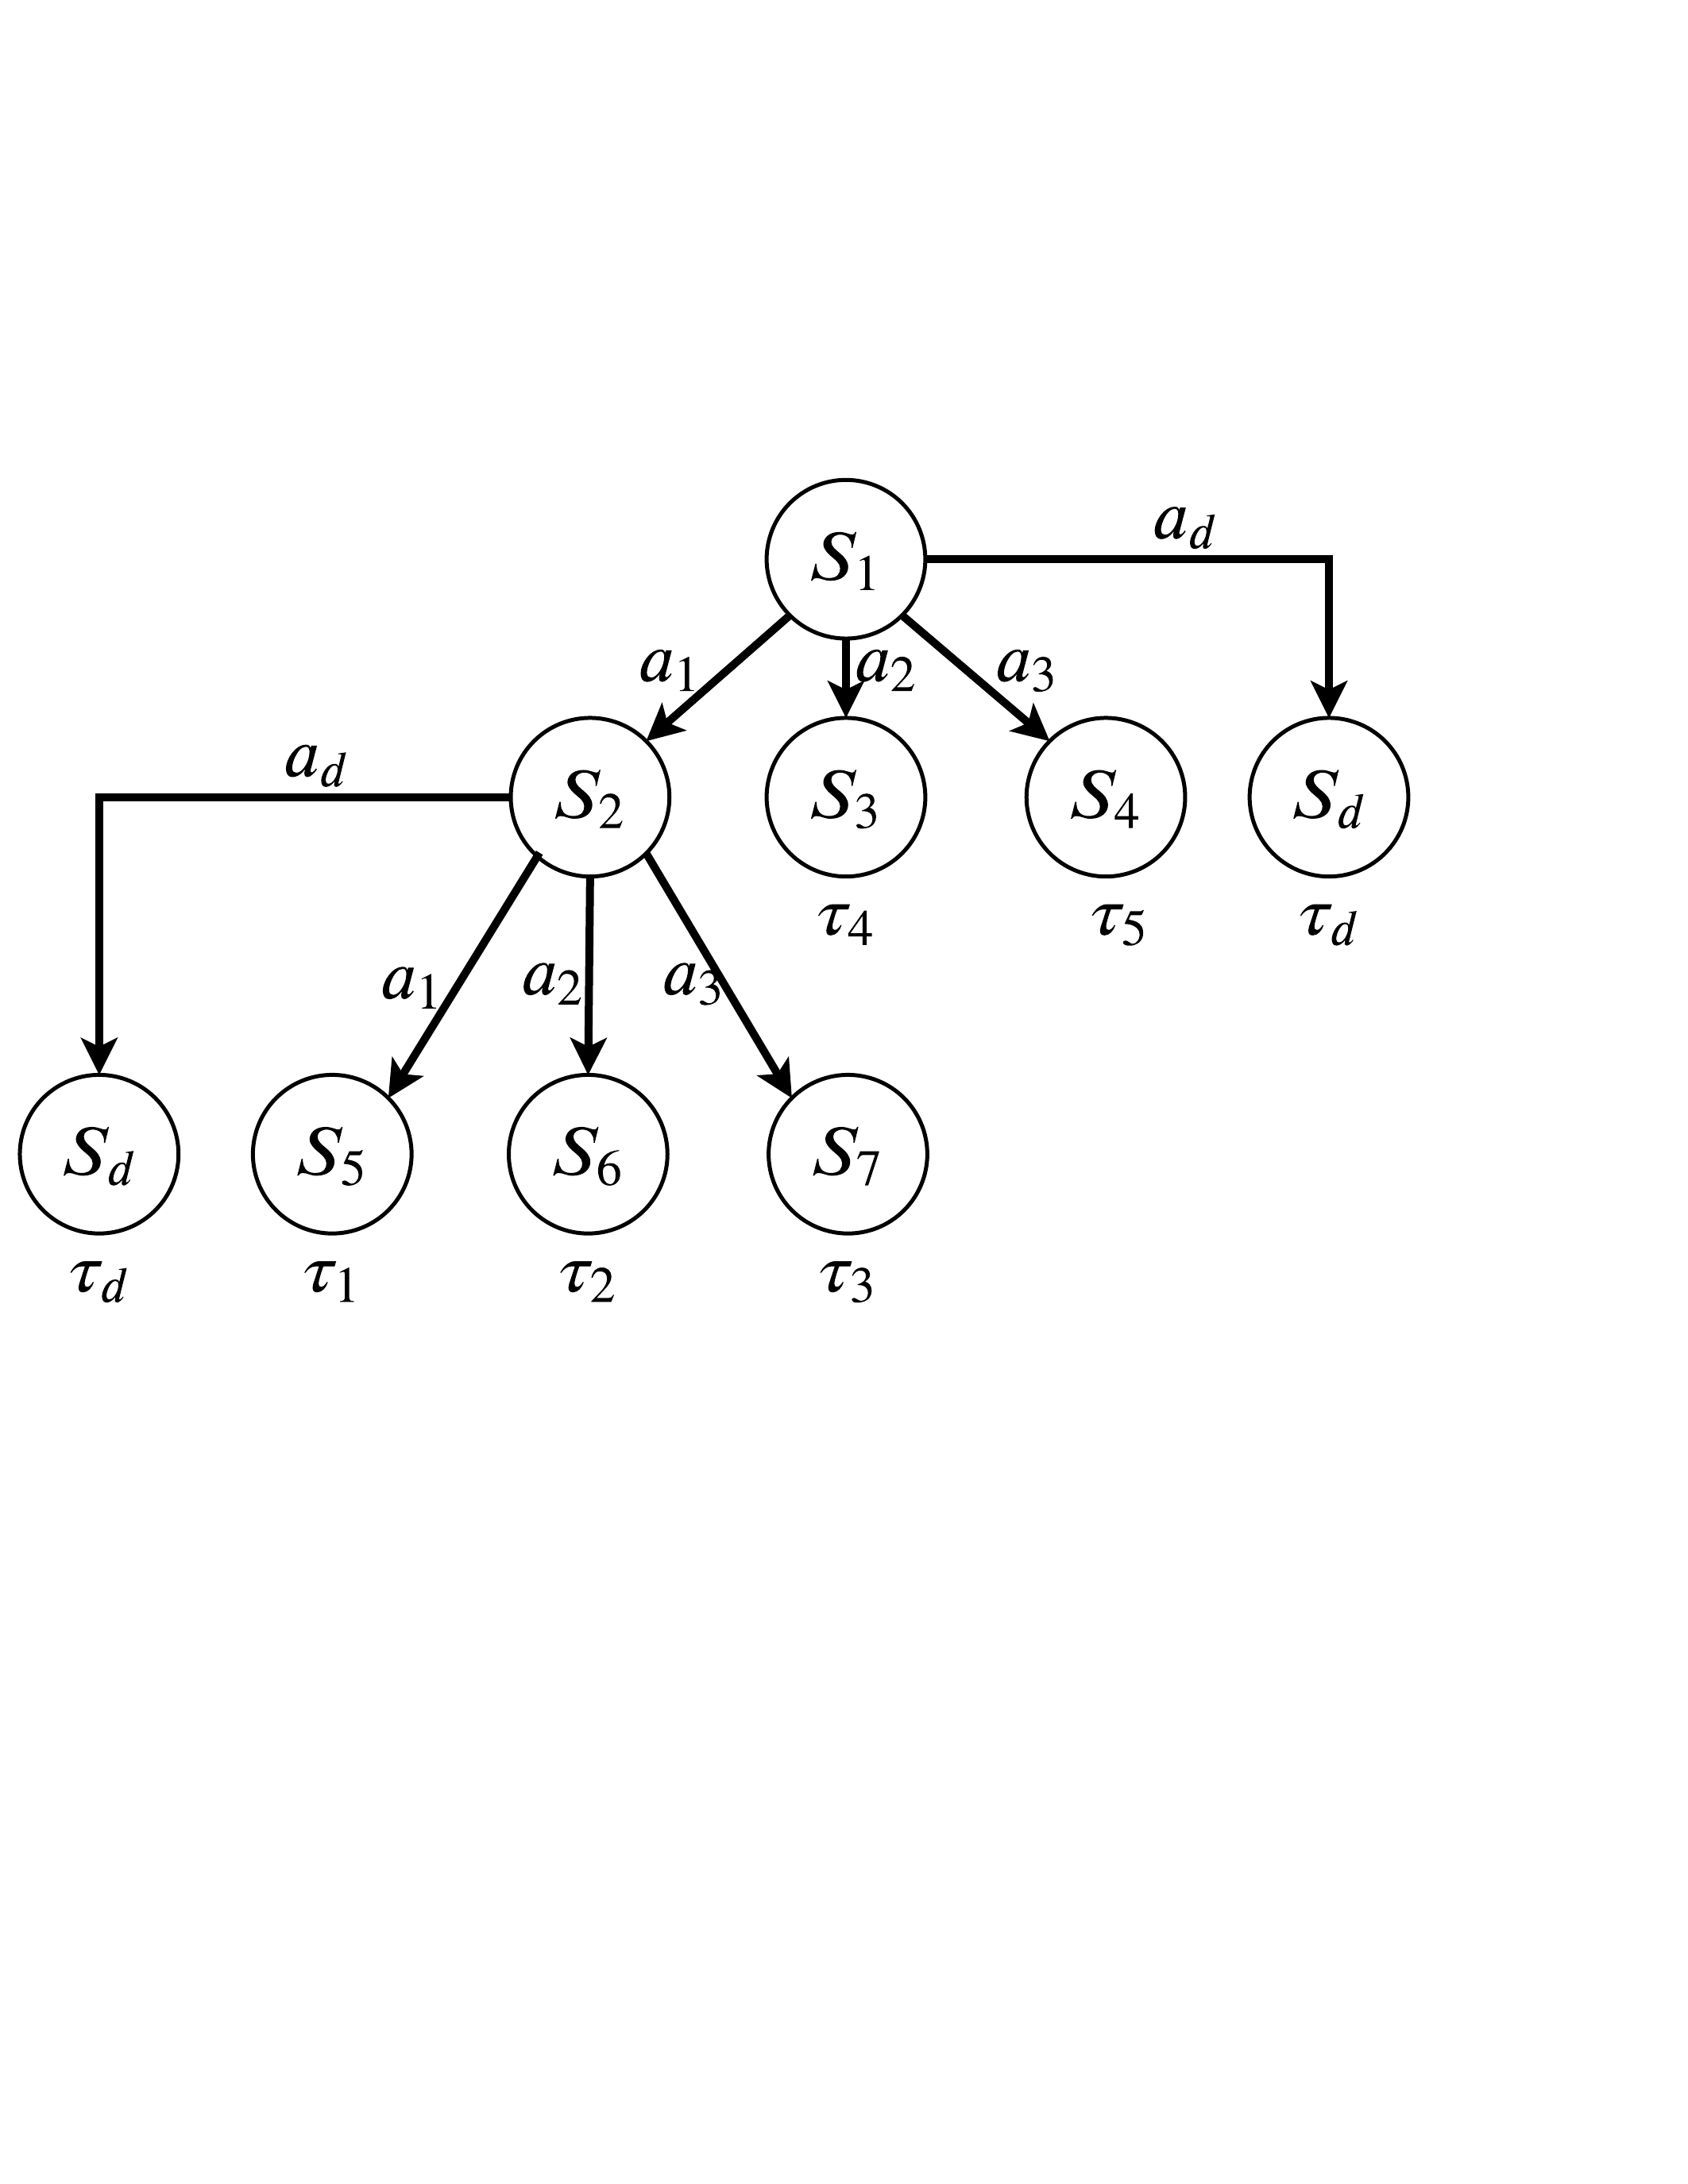}
	\caption{A binary tree MDP consider the dummy action.}
	\label{fig:dummymdp}
\end{figure}
Let's consider a concrete example when $m=3$ in a binary tree MDP, as shown in Figure~\ref{fig:dummymdp}.
Since the $\pi(a_1|s) + \pi(a_2|s) + \pi(a_3|s) < 1$, 
we introduce the dummy action $a_d$, 
where $\pi(a_d|s) = 1 - \sum_i \pi(a_i|s)$. In this case, we have
$\sum_{i=1}^3 \pi(a_i|s) + \pi(a_d|s) = 1$.

The expected reward in this MDP is given as follows:
\begin{align*}
	&\sum_{\tau}\nolimits p_{\theta}(\tau) r(\tau) \\
	=& \sum_{i=1}^5 p_{\theta}(\tau_i) r(\tau_i) + p_{\theta}(\tau_d) r(\tau_d)\\  
	=& \sum_{i=1}^5 p_{\theta}(\tau_i) r(\tau_i) \ (\text{set } r(\tau_d) = 0)\\
\end{align*}
Then the gradient of this expected long term reward is same as 
derivation of \eq{\ref{eq:rlpgobj}}.
