# Supplementary material for: Ranking Policy Gradient
Source: arXiv:1906.09674 source file (2019-11-26)
Supplement: Supplementary file 4 [file sec_appendix_lpg.tex]

% !TEX ROOT=./main.tex

\subsection{Listwise Policy Gradient}
\label{sec:lpgproof}

In order to learn the stochastic policy that optimizes the ranking of actions
with respect to the return, we now introduce the Listwise Policy Gradient (LPG) method.
In RL, we want to optimize the probability of
each action ($a_i$) to be ranked higher among all actions, which is the sum
of the probabilities of all permutations such that the action $a_i$ in the top
position of the list. This probability is computationally prohibitive 
since we need to consider the probability of $m!$ permutations.
Luckily, based on \cite{cao2007learning} [Theorem 6], we can model the
such probability of action $a_i$ to be ranked highest given a set of action values
by a simple softmax formulation, as described in Theorem~\ref{th:top1}.

\begin{theorem}[Theorem 6~\cite{cao2007learning}]
	Given the action values $q=[Q_1,...,Q_m]$, the probability of action $i$ to be taken (i.e. to 
	be ranked on the top of the list) is:
\begin{align}
\pi(a_t=a_i|s_t)= \frac{\phi(Q_i)}{\sum_{j=1}^m {\phi(Q_j)}}
\label{eq:top1:p}	
\end{align}
where $\phi(*)$ is any increasing, strictly positive function. A common choice of $\phi$ is
the exponential function.% with the pro $\phi(x)>0, \ \forall x$.
\label{th:top1}
\end{theorem}
Closely built upon the foundations from learning to
rank~\cite{cao2007learning}, we present the 
listwise policy gradient method, as introduced in
Theorem~\ref{th:lpgt}.
\begin{theorem}[Listwise Policy Gradient Theorem]
For any MDP, the gradient of the long-term reward $J(\theta) = \sum_{\tau} p_{\theta}(\tau) r(\tau)$ w.r.t. 
the parameter $\theta$ of listwise ranking policy takes the following form:
\begin{align}
\grad_{\theta} J({\theta}) = \vE_{\tau \sim \pi_\theta}\left[ \sum_{t=1}^{T}\grad_{\theta} \left( \log \frac{e^{Q_i}}{\sum_{j=1}^m {e^{Q_j}}}\right) r(\tau)\right], 
\label{eq:lpg}
\end{align}
where the listwise ranking policy $\pi_{\theta}$ parameterized by $\theta$ is given by \eq{\ref{eq:lpgt:argmax}} 
for tasks with deterministic optimal policies:
\begin{align}
a = \argmax_{i} Q_i, \quad i=1,\dots,m
\label{eq:lpgt:argmax}
\end{align}
or \eq{\ref{eq:lpgt:sample}} for stochastic optimal policies:
\begin{align}
a \sim \pi(*|s), \quad i=1,\dots,m
\label{eq:lpgt:sample}
\end{align}
where the policy takes the form as in \eq{\ref{eq:lpgt:p}}
\begin{align}
\pi(a=a_i|s_t)= \frac{e^{Q_i}}{\sum_{j=1}^m {e^{Q_j}}}
\label{eq:lpgt:p}	
\end{align}
is the probability that action $i$ being ranked highest, given the current state and all the action values $Q_1 \dots Q_m$.
\label{th:lpgt}
\end{theorem}
The proof of Theorem~\ref{th:lpgt} exactly follows the direct policy differentiation~\cite{peters2008reinforcement,williams1992simple} by replacing the policy to the form of the softmax function. 
The action probability $\pi(a_i|s), \forall i=1,...,m$ forms a probability distribution
over the set of discrete actions [\cite{cao2007learning} Lemma 7]. 
Theorem~\ref{th:lpgt} states that the vanilla policy gradient~\cite{williams1992simple} 
parameterized by a softmax layer is optimizing the 
probability of each action to be ranked highest, with respect to the long-term reward.
